# Supplementary material for: Bayesian spline-based hidden Markov models with applications to actimetry data and sleep analysis
Source: arXiv:2011.01567 source file (2023-10-02)
Supplement: Supplementary file 1 [file supplementary.pdf]

# Appendix to the paper **Bayesian inference for spine-based hidden Markov models**

Sida Chen and Bärbel Finkenstädt Rand  
Department of Statistics, University of Warwick

## **A Further details of the reversible jump MCMC algorithm**

In this section, we give further computational and implementational details related to the reversible jump MCMC algorithm presented in Section 4 and establish the validity of the algorithm.

### **A.1 Acceptance probabilities for the fixed dimensional moves**

Moves (a) and (b) are standard Metropolis-Hastings updates. For (a), the acceptance probability for relocating the knot  $r_{k^*}$  to the candidate point  $r_c$  is:

$$\min\left(1, \frac{f(y^{(n)}|K, R'_K, \tilde{A}_K, \tilde{\delta}, \tilde{\Gamma})f_{N,[a,b]}(r_{k^*}|r_c, \tau_1^2)}{f(y^{(n)}|K, R_K, \tilde{A}_K, \tilde{\delta}, \tilde{\Gamma})f_{N,[a,b]}(r_c|r_{k^*}, \tau_1^2)}\right),$$

where  $R'_K$  differs from  $R_K$  only in the replacement of  $r_{k^*}$  by  $r_c$ , and  $f_{N,[a,b]}(\cdot|\mu, \sigma^2)$  denotes the density of the truncated normal distribution with mean  $\mu$ , standard deviation  $\sigma$  and bounded on  $[a, b]$ . For move (b) since the proposal is symmetric the acceptance probability is:

$$\min\left(1, \frac{f(y^{(n)}|K, R_K, \tilde{A}'_K, \tilde{\delta}, \tilde{\Gamma})f(\tilde{A}'_K|K, \zeta)}{f(y^{(n)}|K, R_K, \tilde{A}_K, \tilde{\delta}, \tilde{\Gamma})f(\tilde{A}_K|K, \zeta)}\right),$$

where the set of  $\tilde{a}'_{i,j}$  is denoted by  $\tilde{A}'_K$ . In steps (c)-(e) we used log-normal random walk to update the parameters due to the positivity constraint, and the corresponding acceptance probabilities for these moves are, respectively,

$$\min \left( 1, \frac{f(\tilde{A}_K|K, \zeta')f(\zeta')\zeta'}{f(\tilde{A}_K|K, \zeta)f(\zeta)\zeta} \right),$$

$$\min \left( 1, \frac{f(y^{(n)}|K, R_K, \tilde{A}_K, \tilde{\delta}', \tilde{\Gamma})f(\tilde{\delta}')}{f(y^{(n)}|K, R_K, \tilde{A}_K, \tilde{\delta}, \tilde{\Gamma})f(\tilde{\delta})} \prod_{i=1}^N \frac{\tilde{\delta}'_i}{\tilde{\delta}_i} \right),$$

and

$$\min \left( 1, \frac{f(y^{(n)}|K, R_K, \tilde{A}_K, \tilde{\delta}, \tilde{\Gamma}')f(\tilde{\Gamma}')}{f(y^{(n)}|K, R_K, \tilde{A}_K, \tilde{\delta}, \tilde{\Gamma})f(\tilde{\Gamma})} \prod_{i=1}^N \prod_{j=1}^N \frac{\tilde{\gamma}'_{i,j}}{\tilde{\gamma}_{i,j}} \right),$$

where  $\tilde{\delta}'$  and  $\tilde{\Gamma}'$  denote the vectors of proposed  $\tilde{\delta}'_i$  and  $\tilde{\gamma}'_{i,j}$ , respectively.

## A.2 Acceptance probabilities for the birth and death moves

Using the notation of Green (1995), the birth move regarding spline parameters is accepted with probability  $\min(1, A)$ , where  $A$  could be expressed in the form

$$\text{likelihood ratio} \times \text{prior ratio} \times \text{proposal ratio} \times \text{Jacobian}.$$

In our context the likelihood ratio is:

$$\frac{f(y^{(n)}|K+1, R_{K+1}, \tilde{A}'_{K+1}, \tilde{\delta}, \tilde{\Gamma})}{f(y^{(n)}|K, R_K, \tilde{A}_K, \tilde{\delta}, \tilde{\Gamma})},$$

where  $\tilde{A}'_{K+1}$  stands for the set of proposed  $\tilde{a}'_{i,j}$  and the likelihood  $f(y^{(n)}|\cdot)$  is given by equation (2). The prior ratio is given by the product of the ratio of the priors on each block of parameters that are involved in this update:

$$\frac{f_U(K+1)}{f_U(K)} \frac{\frac{(K+1)!}{(b-a)^{K+1}} \prod_{i=1}^N \prod_{j=1}^{K+5} f_{LG}(\tilde{a}'_{i,j}|\zeta, 1)}{\frac{K!}{(b-a)^K} \prod_{i=1}^N \prod_{j=1}^{K+4} f_{LG}(\tilde{a}_{i,j}|\zeta, 1)}$$

where  $f_U(\cdot)$  denotes the probability mass function of a uniformly distributed random variable on  $\{2, \dots, K_{\max}\}$  and  $f_{LG}(\cdot|\zeta, 1)$  stands for the log-gamma density with shape parameter  $\zeta$  and rate parameter 1. The proposal ratio is given by

$$\frac{d_{K+1}}{(K+1)} \left\{ b_K \frac{\sum_{i=1}^K f_{N,[a,b]}(r_c|r_i, \tau(R_K, i)^2)}{K} \right\}^{-1},$$

where  $f_{N,[a,b]}(\cdot|\mu, \sigma^2)$  denotes the density of a truncated normal distribution with mean  $\mu$ , standard deviation  $\sigma$  and bounded on  $[a, b]$ . Lastly, the Jacobian corresponding to the transformation from  $(R_K, \tilde{A}_K, \tilde{\delta}, \tilde{\Gamma}, r_c, u_1, \dots, u_N)$  to  $(R_{K+1}, \tilde{A}'_{K+1}, \tilde{\delta}, \tilde{\Gamma})$  is

$$|(r_{n^*+2}r_{n^*+3})^N \prod_{i=1}^N (\tilde{a}_{i,n^*+4} - \tilde{a}_{i,n^*+3})|.$$

After simplification  $A$  is thus given by

$$A = \frac{f(y^{(n)}|K+1, R_{K+1}, \tilde{A}'_{K+1}, \tilde{\delta}, \tilde{\Gamma})}{f(y^{(n)}|K, R_K, \tilde{A}_K, \tilde{\delta}, \tilde{\Gamma})} \frac{1}{(b-a)} \frac{\prod_{i=1}^N \prod_{j=n^*+2}^{n^*+4} f_{LG}(\tilde{a}'_{i,j}|\zeta, 1)}{\prod_{i=1}^N \prod_{j=n^*+2}^{n^*+3} f_{LG}(\tilde{a}_{i,j}|\zeta, 1)} \\ \times \frac{d_{K+1}}{b_K} \left\{ \frac{\sum_{i=1}^K f_{N,[a,b]}(r_c|r_i, \tau(R_K, i)^2)}{K} \right\}^{-1} |(r_{n^*+2}r_{n^*+3})^N \prod_{i=1}^N (\tilde{a}_{i,n^*+4} - \tilde{a}_{i,n^*+3})|.$$

Since the birth and death moves are defined in a symmetric way, the acceptance probability for this death move is  $\min(1, A^{-1})$ , where  $K$  is replaced by  $K-1$  and  $n^* = d^* - 1$ .

### A.3 Validity of the algorithm

The validity of the proposed reversible jump MCMC algorithm can be established following standard results in Tierney (1994) and Robert and Casella (2013). First note that the Markov transition kernel for each of the move steps admits the target posterior distribution,  $f$  (defined through equation (3)), as invariant distribution, so a concatenation of these kernels also admits  $f$  as invariant distribution. Irreducibility of the constructed chain can be deduced as the chain can move from one value of  $K$  to any other possible value by increasing or decreasing its value by one at a time, with positive probability. In steps (b), (d) and (e) the proposal density is positive on the natural parameter space and the same holds true for step (a) if we consider several consecutive sweeps. The chain is also aperiodic as there is a strictly positive probability that the chain remains in a neighbourhood of the current state after one sweep of the MCMC procedure. With the above properties the chain is guaranteed to converge to the posterior distribution from almost all initial states (except for a set of posterior probability zero). To replace "almost all" by "all" we require a stronger condition called Harris recurrence, which is generally difficult to verify in the trans-dimensional MCMC set-up (Roberts and Rosenthal, 2006; Hastie and Green, 2012).

However in practice we could tackle this issue by drawing the initial state using a continuous distribution centered around the posterior mode (or other approximations to that such as the maximum likelihood estimate). This strategy is employed in our initialization process. To accelerate the convergence of the chain we initialize the knot points at the empirical quantiles of the data so that more knots are initially placed at data-rich regions. For the remaining parameters the initial values are drawn from appropriate truncated normal distributions centered at their respective maximum likelihood estimates computed given the initial knot configuration.

## A.4 Tackling label switching

A practical consequence of the properties of the model and its prior is that samples generated by the reversible jump MCMC algorithm are subject to the label switching problem, i.e. the state labels can permute during the MCMC iterations without changing the posterior density. As a result, the MCMC output cannot be directly used for inference about the state specific parameters. To tackle this issue we choose to use the pivotal reordering technique suggested in Marin et al. (2005) and Spezia (2009). More details and comparative review of alternative solutions to this problem can be found therein. An outline of the procedure is as follows. We first run the algorithm in an unconstrained way as proposed above and the knot configuration, which is unaffected by label switching, is estimated at the end of the sampling process as  $\hat{K} = \operatorname{argmin}_K \hat{P}(K|y)$  and  $\hat{R}_K = \frac{\sum_{i=1}^T \mathbf{I}(K^{(i)}=\hat{K}) R_{K^{(i)}}}{\sum_{i=1}^T \mathbf{I}(K^{(i)}=\hat{K})}$ , where  $\hat{P}(K|y)$  is directly estimated from the reversible jump MCMC output and  $T$  is the size of the MCMC samples (not including burn-in). Conditioned on  $\hat{K}$ , the state labels of each MCMC samples are reordered such that its Euclidean distance to the sample-based maximum a posteriori (MAP) estimate of the parameters with  $K = \hat{K}$ ,  $\left\| \eta_j(\Theta^{(k)}) - \Theta_{\hat{K}}^{MAP} \right\|$ , where  $\eta_j(\cdot)$  is some permutation of the state-specific parameters and  $j = 1, \dots, N!$ , is minimized. The reordered samples can then be used for posterior inference. However, this method may run into problems when the state-specific (spline) coefficients are similar (i.e. the emission densities are highly overlapping), as we did encounter for the third simulation model (the trimod model). To better distinguish between different possibilities of the state

labels, we propose to consider the 'distance' between the emission densities induced by  $\eta_j(\Theta^{(k)})$  and  $\Theta_{\hat{K}}^{MAP}$ , i.e.

$$\left\| \mathbf{f}_{\eta_j}^{(k)} - \mathbf{f}^{MAP} \right\|, \quad (9)$$

where  $\mathbf{f}_{\eta_j}^{(k)} = (f_{\eta_j^1}^{(k)}(y^{(1)}), \dots, f_{\eta_j^1}^{(k)}(y^{(n)}), \dots, f_{\eta_j^N}^{(k)}(y^{(1)}), \dots, f_{\eta_j^N}^{(k)}(y^{(n)}))$ ,  $\mathbf{f}^{MAP} = (f_1^{MAP}(y^{(1)}), \dots, f_1^{MAP}(y^{(n)}), \dots, f_N^{MAP}(y^{(1)}), \dots, f_N^{MAP}(y^{(n)}))$ . The  $f_{\cdot}^{(k)}(\cdot)$  and  $f_{\cdot}^{MAP}(\cdot)$  are given by equation (1), constructed via the  $k$ -th sample and the MAP sample, respectively. Thus for the  $k$ -th sample we seek a specific permutation  $\eta_{j*} = (\eta_{j*}^1, \dots, \eta_{j*}^N)$  of the state labels such that (9) is minimised. Our experience suggests that in this challenging scenario it often acts more effectively in finding the "correct" state labels than the original pivotal reordering algorithm.

## B Additional results for the simulation study

In this section we give more details and discuss the performance of the proposed algorithm for our simulation models presented in Section 4. The settings for some unspecified constants used in the algorithm are given in Table 1, whose values were tuned via short pilot runs on the simulated data sets. Some diagnostic plots that are related to the mixing and convergence of the sampler are shown in Figures B.1, B.2 and B.3, where the results for each model are obtained for a randomly selected replication of the simulated data set.

For fixed dimensional moves (moves (a)-(e)), the acceptance rates are controlled at the level of 25% – 40%. We analyzed the traces and running averages for selective parameters across MCMC iterations and found satisfactory mixing patterns in most cases. For the dimension changing moves, the averaged acceptance rates for models 1, 2 and 3 are 0.31%, 0.15%, 0.77% ( $n = 1000$ ) and 0.35% ( $n = 5000$ ), respectively. While it is lower than desired in our simulation cases, we did not detect any apparent convergence issues (see Figures B.1, B.2 and B.3). For Model 2 the acceptance rate can be expected to be lower than for the other two scenarios as it has a larger number of states whose emission distributions have quite different characteristics. In general, a new knot is more likely to be accepted if it contributes to some extent to the fit of all the emission densities. On the other hand, the

Table 1: Constants used for the reversible jump MCMC algorithm.

| Model      | a                    | b                    | $\tau_1$ | $\tau_2$ | $\tau_3$ | $\tau_4$ | $\tau_5$ | $\alpha$ |
|------------|----------------------|----------------------|----------|----------|----------|----------|----------|----------|
| 1          | $\min(y^{(n)}) - 10$ | $\max(y^{(n)}) + 10$ | 8        | 0.24     | 0.7      | 2        | 0.24     | 0.65     |
| 2          | $\min(y^{(n)}) - 10$ | $\max(y^{(n)}) + 10$ | 9        | 0.15     | 0.5      | 1.8      | 0.17     | 0.65     |
| 3 (n=1000) | $\min(y^{(n)}) - 5$  | $\max(y^{(n)}) + 5$  | 0.8      | 0.11     | 0.5      | 2        | 0.65     | 0.65     |
| 3 (n=5000) | $\min(y^{(n)}) - 5$  | $\max(y^{(n)}) + 5$  | 0.6      | 0.05     | 0.6      | 2        | 0.5      | 0.65     |

degree of precision in the posterior distribution of  $K$  is limiting the achievable acceptance rates for the dimension changing moves. For instance, as  $n$  increases, the posterior for  $K$  is expected to be more concentrated, leading to a generally lower acceptance rate. From the algorithmic perspective this rate is mildly affected by the standard deviation  $\tau$  of the truncated normal distribution or the proposal distribution for  $u_i$  used in the birth move. With the functional form of  $\tau$  fixed, we tested the algorithm for a number of choices of  $\alpha$ , among which those given in Table 1 performed best. We also investigated the use of other potential proposal distributions in the Beta family, but no clear evidence was found in terms of their superiority over the choice  $U(0, 1)$ . A higher acceptance rate for the dimension changing move may be achieved by modifying the current model or the proposal mechanism. For instance, one might consider using a separate knot configuration for each emission density and propose state-specific jump moves, or generating the random variables  $u_i$  used in equation (5) from a more informative proposal distribution such as a truncated normal distribution centred at its maximum likelihood estimate. However, in either scenario the model complexity or the computational effort may increase significantly, which may prevent a successful application of the algorithm in some settings. Though not presented here, we also investigated the estimation performance of the algorithm with other simulation settings. Our preliminary findings indicate that the performance generally improves as serial correlation and/or sample size increases, while it declines as the number of states and/or the overlap of the emission distributions increases.

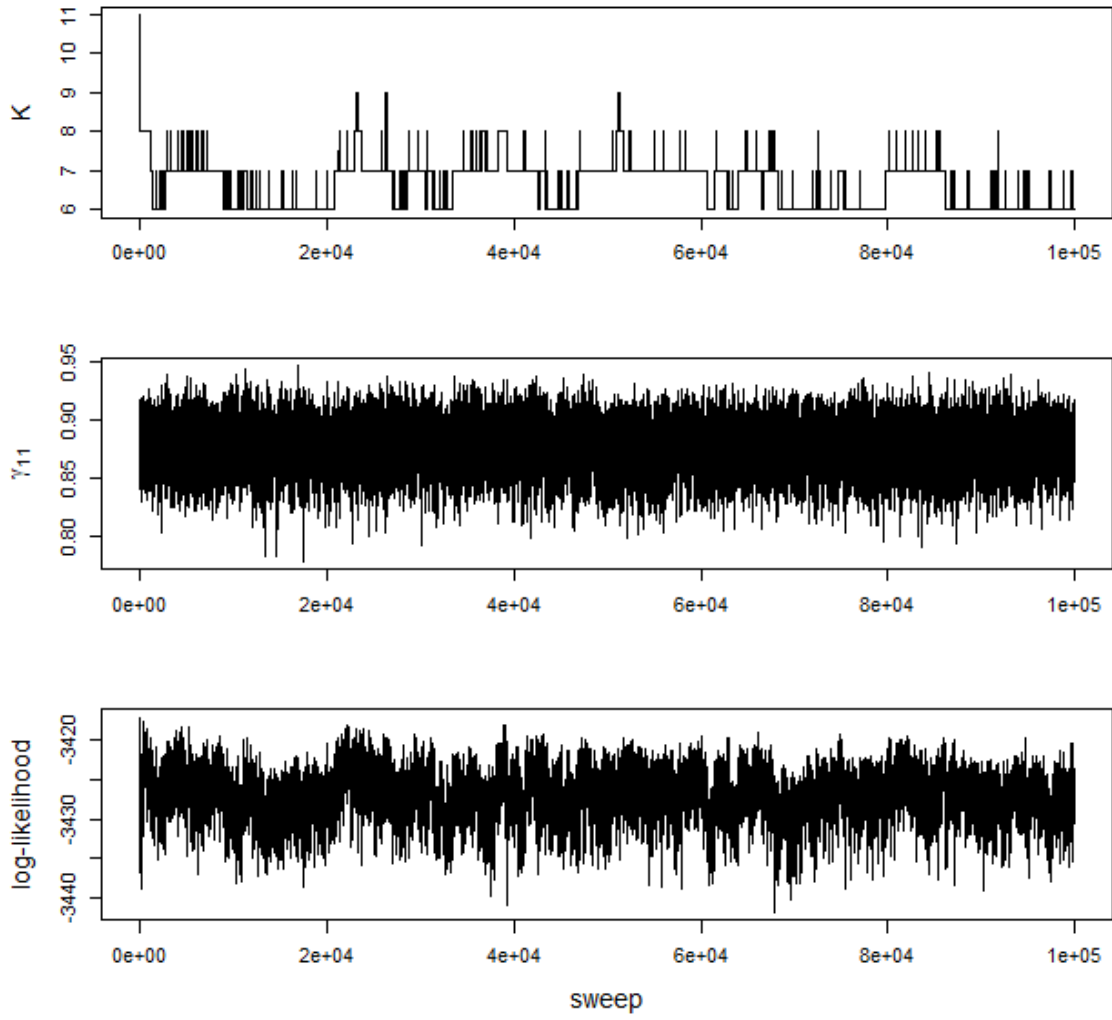

Figure B.1: Results for simulation model 1 conditioned on  $N = 2$ . Top panel: trace of  $K$  for a complete run of 100k MCMC iterations including burn in; middle panel: the corresponding trace for  $r_{11}$  across MCMC iterations; bottom panel: the corresponding log-likelihood of the model generated by the algorithm.

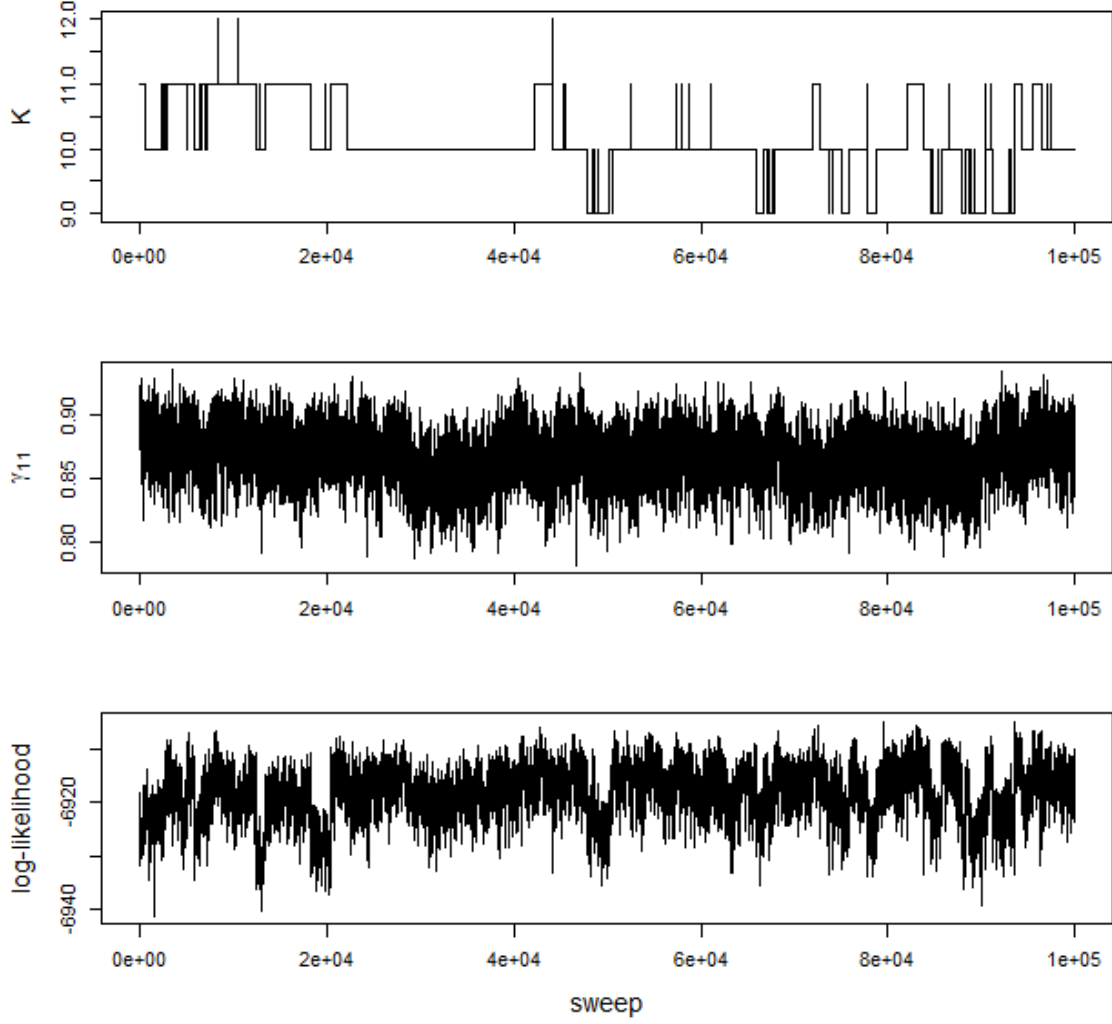

Figure B.2: Results for simulation model 2 conditioned on  $N = 3$ . Top panel: trace of  $K$  for a complete run of 100k MCMC iterations including burn in; middle panel: the corresponding trace for  $r_{11}$  across MCMC iterations; bottom panel: the corresponding log-likelihood of the model generated by the algorithm.



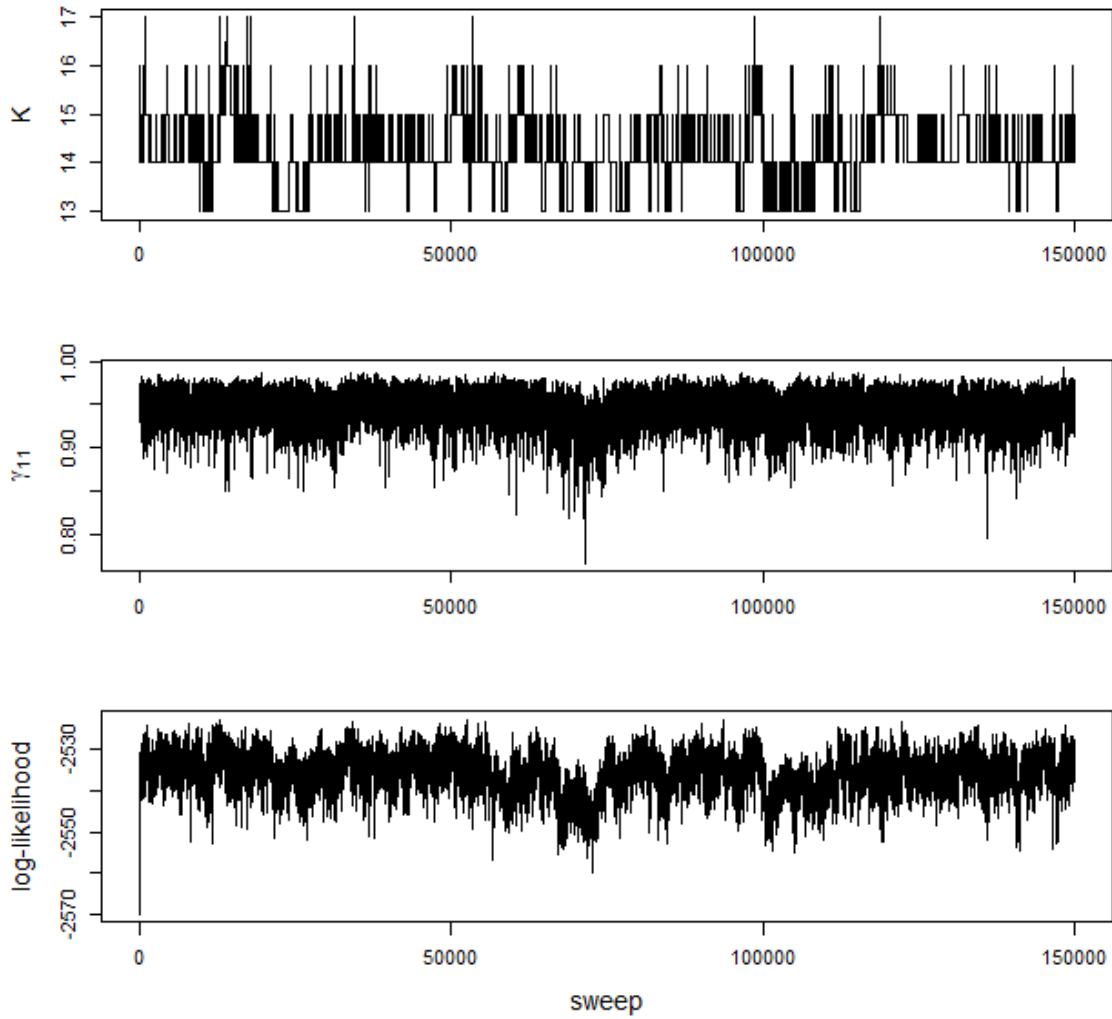

Figure B.3: Results for simulation model 3 ( $n = 1000$ ) conditioned on  $N = 2$ . Top panel: trace of  $K$  for a complete run of 100k MCMC iterations including burn in; middle panel: the corresponding trace for  $r_{11}$  across MCMC iterations; bottom panel: the corresponding log-likelihood of the model generated by the algorithm.

## C Further details of the empirical application of Section 6.1

In this section we provide additional details for the 3 and 7-state HMMs estimated by our proposed method. For the 3-state model, our posterior summaries for the entries of the transition probability matrix are

$$\hat{\Gamma} = \begin{pmatrix} 0.943_{(0.006)} & 0.057_{(0.006)} & 0.001_{(0.001)} \\ 0.029_{(0.003)} & 0.961_{(0.004)} & 0.01_{(0.002)} \\ 0.005_{(0.004)} & 0.048_{(0.01)} & 0.947_{(0.01)} \end{pmatrix},$$

where the point estimates are the posterior means and the associated standard deviations are shown in brackets. In particular, the diagonal entries of  $\hat{\Gamma}$  are all close to 1 highlighting the serial dependence. For the 7-state model, our posterior estimates are based on 50k draws after a burn-in of 50k iterations. Figure C.1 displays the estimated emission densities (left panel) and the Viterbi-decoded times series (right panel) obtained based on posterior means of the model's parameter vector with  $K$  fixed to its posterior mode. We can see that the estimated hidden states roughly correspond to 7 different levels of activity which resolves the multimodality seen in the 3-state model (state 1) into a mixture of unimodal emission densities. Posterior means for the transition probabilities are

$$\hat{\Gamma}_7 = \begin{pmatrix} 0.863 & 0.118 & 0.008 & 0.003 & 0.003 & 0.002 & 0.002 \\ 0.068 & 0.777 & 0.135 & 0.008 & 0.004 & 0.008 & 0.001 \\ 0.017 & 0.117 & 0.69 & 0.137 & 0.02 & 0.017 & 0.002 \\ 0.001 & 0.002 & 0.059 & 0.791 & 0.134 & 0.012 & 0.001 \\ 0.001 & 0.004 & 0.012 & 0.102 & 0.83 & 0.05 & 0.001 \\ 0.004 & 0.019 & 0.047 & 0.038 & 0.072 & 0.775 & 0.045 \\ 0.002 & 0.003 & 0.003 & 0.002 & 0.003 & 0.052 & 0.935 \end{pmatrix}.$$

All of the estimated states are persistent in the sense that there usually is a large probability of staying in the current state (see diagonal entries of  $\hat{\Gamma}_7$ ). In comparison to the 3-state model, the diagonal entries are naturally lower as the shark's movement is now sub-divided into more states. The fitted model with 7 states indicates, for example, that the lower

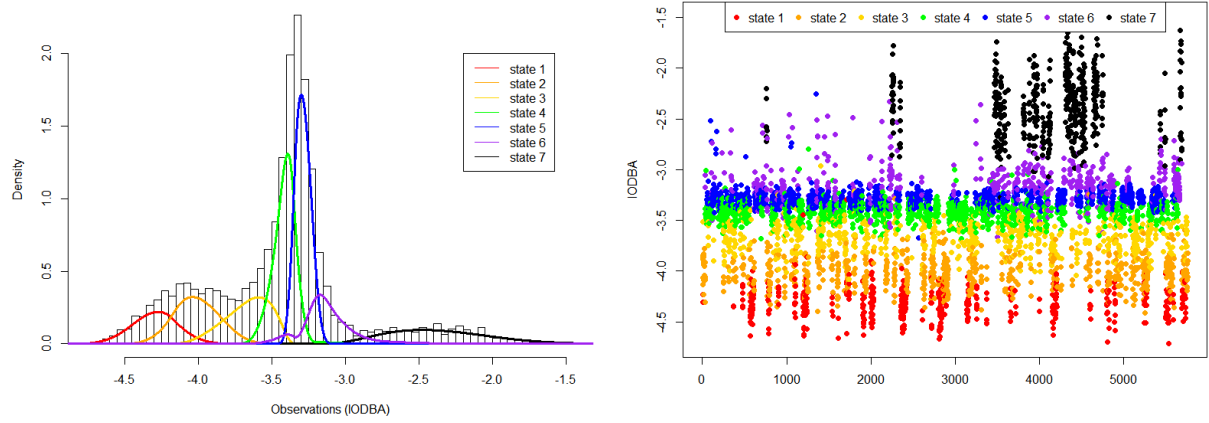

Figure C.1: Left panel: histogram of 15s-averaged IODBA values along with the estimated emission densities (weighted according to their proportion in the stationary distribution of the estimated Markov chain) obtained from our method; right panel: the corresponding Viterbi-decoded time series conditional on the posterior estimate of the parameter of the 7-state model. Here the state labels are sorted according to their mean IODBA levels.

and middle activity mode of the 3-state model can each be associated to several separate states, while the higher activity mode still corresponds to a single state, state 7, whose onset typically occurs following state 6. To assign biologically meaningful interpretations to these states, however, additional specialized information is required and we shall not pursue it further here. Nevertheless, our analysis demonstrates the ability of our method of dealing with model selection in an HMM with a relatively large number of states, while Langrock et al.'s approach may be severely challenged with increasing  $N$ . We also notice that the emission densities of the 7-state model has a fairly regular shape, thus our nonparametric approach could be used in an explorative way to identify a suitable parametric model.

## D Further details of the empirical application of Section 6.2

In this section we present additional implementation details and estimation results for applying the proposed conditional HMM approach on the example subject (subject 9 in Section 6.2).

### D.1 The main HMM

Posterior simulation for the main model can be achieved by using the same MCMC methodology described in Section 3, augmented with an additional Metropolis-Hastings step to update state-specific zero weights  $w_i$ . More specifically, we reparameterize the weights as

$$w_{i,j} = \frac{\tilde{w}_{i,j}}{\tilde{w}_{i,1} + \tilde{w}_{i,2}}, \quad \tilde{w}_{i,j} > 0,$$

where  $w_{i,1}$  corresponds to the probability of observing zero for state  $i$ ,  $i = 1, \dots, N$ ,  $j = 1, 2$ . We choose a vague gamma prior on the  $\tilde{w}_{i,j}$ , i.e.  $f(\tilde{w}_{i,j}) = \text{gamma}(1, 1)$ , which gives a  $\text{Dir}(1, 1)$  distribution on  $(w_{i,1}, w_{i,2})$ . In the MCMC algorithm the  $\tilde{w}_{i,j}$  are updated via a log-normal random walk

$$\log(\tilde{w}'_{i,j}) = \log(\tilde{w}_{i,j}) + \phi_{i,j},$$

where  $\phi_{i,j} \sim \mathcal{N}(0, \tau_6^2)$ . The move is accepted with probability

$$\min\left(1, \frac{f(y^{(n)}|K, R_K, \tilde{A}_K, \tilde{\delta}, \tilde{\Gamma}, \tilde{w}')f(\tilde{w}')}{f(y^{(n)}|K, R_K, \tilde{A}_K, \tilde{\delta}, \tilde{\Gamma}, \tilde{w})f(\tilde{w})} \prod_{i=1}^N \prod_{j=1}^2 \frac{\tilde{w}'_{i,j}}{\tilde{w}_{i,j}}\right),$$

where  $\tilde{w}'$  and  $\tilde{w}$  denote the vectors of proposed  $\tilde{w}'_{i,j}$  and  $\tilde{w}_{i,j}$ , respectively.

In our example, hyperparameters of the prior distributions are specified as  $\epsilon_1 = \epsilon_2 = 1$ ,  $a = 0.1$  and  $b = 362.4$ . Other constants used in the algorithm are taken as  $\tau_1 = 13$ ,  $\tau_2 = 0.3$ ,  $\tau_3 = 0.6$ ,  $\tau_4 = 1.8$ ,  $\tau_5 = 0.22$ ,  $\tau_6 = 0.3$  and  $\alpha = 0.65$  after conducting a few test runs. Our results are based on 50k sweeps of the MCMC algorithm after a burn-in of 50k sweeps. Conditioned on the selected number of states ( $N = 3$ ), the posterior modal number of knots is 6, with  $\hat{P}(K = 6|data) = 0.924$ , and the estimated emission densities (on the positive domain) are displayed in Figure D.1, where the knot sequence and the associated

spline coefficients are estimated by their posterior averages conditional on  $K = 6$ . Our posterior summaries for entries of the transition probability matrix are

$$\hat{\Gamma} = \begin{pmatrix} 0.977_{(0.008)} & 0.02_{(0.008)} & 0.003_{(0.003)} \\ 0.028_{(0.01)} & 0.856_{(0.023)} & 0.116_{(0.021)} \\ 0.004_{(0.003)} & 0.086_{(0.016)} & 0.91_{(0.017)} \end{pmatrix},$$

where the point estimates are the posterior means and the associated standard deviations are shown in brackets.

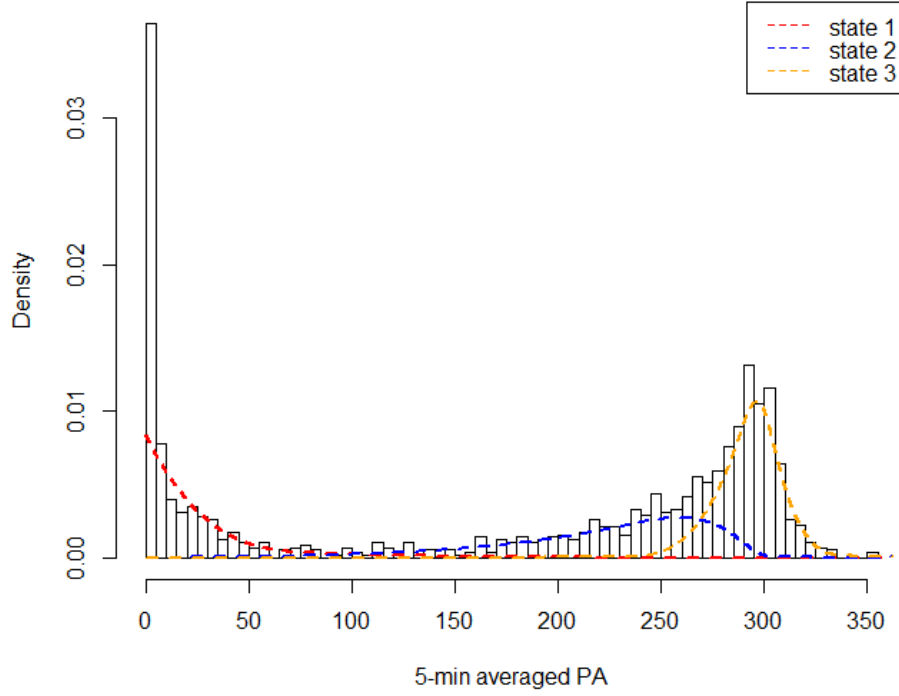

Figure D.1: Histogram of 5-min averaged PA data along with the estimated emission densities (weighted according to their proportion in the stationary distribution of the estimated Markov chain) obtained from our method. The weights at zero for state 1, 2 and 3 are 0.421, 0.003 and 0.002, respectively (not shown in the graph).

## D.2 The sub-HMM

For the sub-HMM, we used the same updating scheme used for the main HMM to update the model parameters including zero weights for each sub-state, and details are omitted here. Hyperparameters of the prior distributions are specified as  $\epsilon_1 = \epsilon_2 = 1$ ,  $a = 1$  and  $b = 323$ . Other constants used in the algorithm are taken as  $\tau_1 = 9$ ,  $\tau_2 = 0.2$ ,  $\tau_3 = 0.7$ ,  $\tau_4 = 1.5$ ,  $\tau_5 = 0.24$ ,  $\tau_6 = 0.25$  and  $\alpha = 0.65$ . Our results are based on 25k samples of  $\Theta_2$  with the first 25k samples discarded as burn-in. The posterior modal number of knots is 3, with posterior probability of 0.97. The estimated emission densities (on the positive domain) for the two sub-states are displayed in Figure D.2, where the knot sequence and the associated spline coefficients are estimated by their posterior averages conditional on  $K = 3$ . Figure D.3 displays the times series of the 1-min position data (measured as the angle formed between the vertical axis and subject's upper body) for each night's sleep bout with colors indicating the Viterbi decoded sub-states from the fitted sub-HMM at each time point. We can see that the occurrences of sub-state 1.2 often coincide with changes in body position.

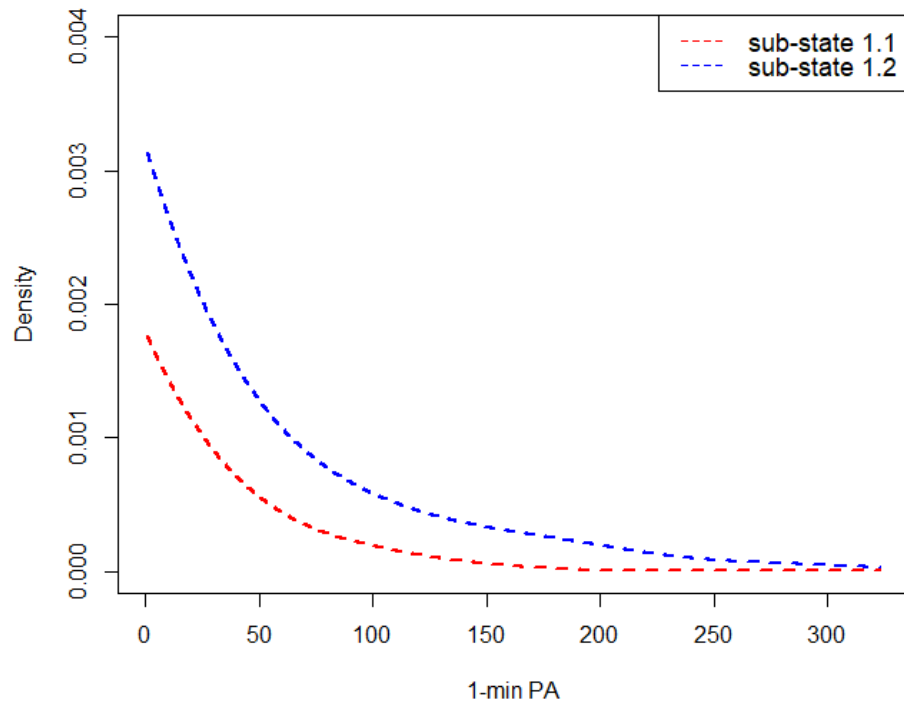

Figure D.2: Estimated emission densities (weighted according to their proportion in the stationary distribution of the estimated Markov chain) obtained from our method. The weights at zero for sub-state 1.1 and 1.2 are 0.898 and 0.246, respectively (not shown in the graph).

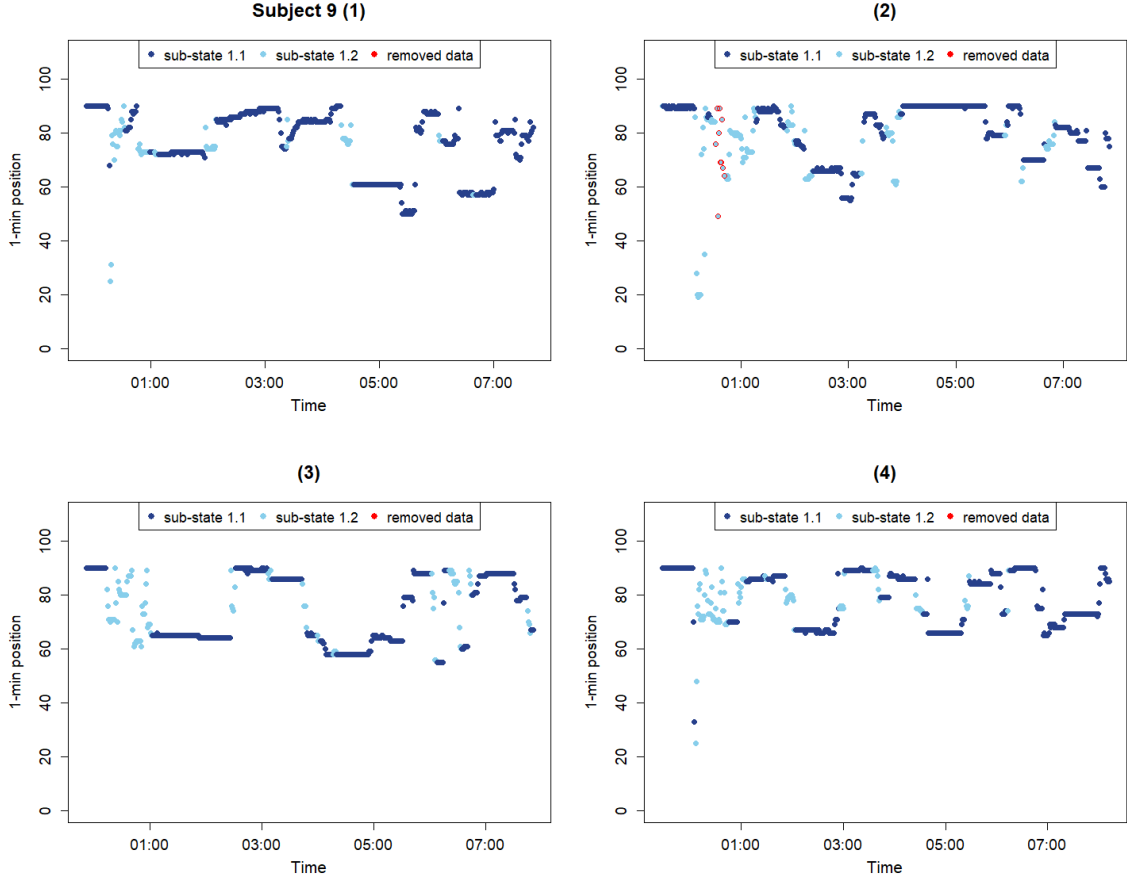

Figure D.3: Panels (1)-(4) display the times series of the 1-min position data for each night's sleep bout with colors indicating the Viterbi decoded sub-states from the fitted sub-HMM at each time point. Removed data (in red) are those that are assigned to a more active state instead of state 1 by the fitted main HMM.



# References

- Green, P. J. (1995). Reversible jump Markov chain Monte Carlo computation and Bayesian model determination. *Biometrika*, 82(4):711–732.
- Hastie, D. I. and Green, P. J. (2012). Model choice using reversible jump Markov chain Monte Carlo. *Statistica Neerlandica*, 66(3):309–338.
- Marin, J.-M., Mengersen, K., and Robert, C. P. (2005). Bayesian modelling and inference on mixtures of distributions. *Handbook of statistics*, 25:459–507.
- Robert, C. and Casella, G. (2013). *Monte Carlo statistical methods*. Springer Science & Business Media.
- Roberts, G. O. and Rosenthal, J. S. (2006). Harris recurrence of metropolis-within-gibbs and trans-dimensional Markov chains. *The Annals of Applied Probability*, pages 2123–2139.
- Spezia, L. (2009). Reversible jump and the label switching problem in hidden Markov models. *Journal of Statistical Planning and Inference*, 139(7):2305–2315.
- Tierney, L. (1994). Markov chains for exploring posterior distributions. *the Annals of Statistics*, pages 1701–1728.
